# Supplementary material for: An Analysis of Super-Net Heuristics in Weight-Sharing NAS
Source: arXiv:2110.01154 source file (2021-10-04)
Supplement: Supplementary file 1 [file appendix.tex]

\appendices

\section{Searching without topology}
\label{apdx:nb101-chain}
\changed{
Apart from DARTS-like search spaces that allow to search for both topology wiring and operations, chain-like linear search spaces~\cite{wu_fbnet:_2018,cai2018proxyless} have been shown to be effective for many computer vision tasks. Since there exists no benchmark linear search space, we construct a linear search space from NASBench 101 (see Figure \ref{fig:nb101-linear}) to study if our findings also hold in this setting. }
\begin{figure}
    \centering
        % \vspace{-.4cm}
    \resizebox{0.7\linewidth}{!}{
    \includegraphics{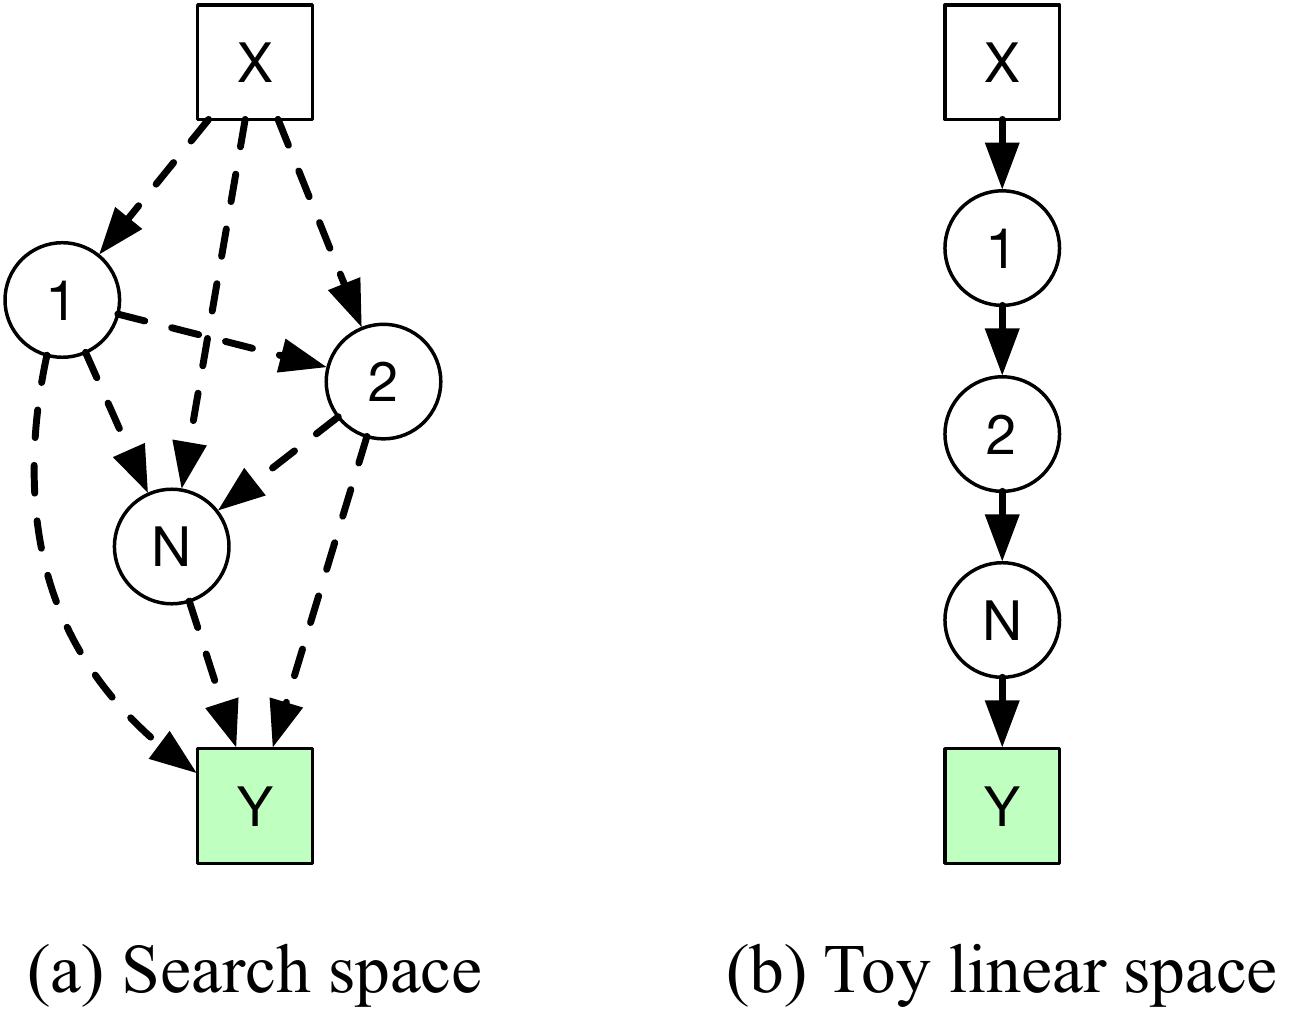}
    }
    \caption{\textbf{Simplifying NASBench-101 to a linear search space.} (a) The original NASBench-101 is a general direct acyclic graph (DAG) search space that each node can be connected to all previous nodes. (b) To mimic a linear search space like MobileNet~\cite{wu_fbnet:_2018} we ensure that each node is only connected to its predecessor. As a consequence, the search is reduced only to operations for each node. This toy search space has 243 architectures in total. 
    }
    \vspace{-0.4cm}
    \label{fig:nb101-linear}
\end{figure}

\changed{
Tables~\ref{tab:pws-nasbench101-linear} and ~\ref{tab:supp-lowfd-nb101-linear} show the results, which indicate that our findings also hold in this linear space.}

\section{Implementation.}
\label{apdx:misc}

\mypara{Implementation Details of \skdt{}.}
To compute the \skdt{} we need access to two quantities: 1) the performance of the sampled architectures based on the trained super-net; and 2) the associated ground-truth performances. For each architecture in 1), we compute the average top-1 accuracy over $n=3$ 
super-nets (that where trained with different random initialization) to improve the stability of the evaluation. We round the ground-truth top-1 accuracy to a precision of 0.1$\%$ for each sampled architecture to obtain the ground-truth performance 2). We then rank the architectures in 1) and 2) and compute the Kendall-Tau rank coefficient \cite{Kendall1938} between the two ranked lists.

% Table~\ref{tab:supp-lowfd-nb101-linear}
% Table~\ref{tab:pws-nasbench101-linear}

\begin{table}[!ht]
    \centering
    \caption{\textbf{Results for all WS Protocol $P_{ws}$ factors on the NASBench-101 linear space.}} 
    \vspace{-0.3cm}
    \resizebox{\linewidth}{!}{
        \begin{tabular} { l|cccc}
        \midrule[2pt]
        Factor & \multicolumn{4}{c}{NASBench-101 linear space} \\
        and &  & Super-net & & Final \\
        settings & Accuracy & S-KdT & P $>$ R &  Performance\\
        \midrule[1pt]
        \multicolumn{3}{l}{\textbf{Batch-norm}} \\
        \midrule
affine F track F &0.478$\pm$0.04&0.131&0.960&0.866$\pm$0.01\\
affine T track F &0.487$\pm$0.07&0.146&0.542&0.852$\pm$0.02\\
affine F track T &0.103$\pm$0.01&-0.154&0.263&0.855$\pm$0.01\\
affine T track T &0.111$\pm$0.02&-0.121&0.651&0.857$\pm$0.01\\
        \midrule[1pt]
        \multicolumn{3}{l}{\textbf{Learning rate}} \\
        \midrule
0.001 &0.188$\pm$0.08&0.363&0.636&0.869$\pm$0.01\\
0.005 &0.515$\pm$0.09&0.558&0.828&0.867$\pm$0.01\\
0.01 &0.570$\pm$0.03&0.233&0.920&0.853$\pm$0.02\\
0.025 &0.568$\pm$0.05&0.160&0.194&0.848$\pm$0.01\\
0.1 &0.655$\pm$0.05&0.168&0.696&0.860$\pm$0.02\\
0.15 &0.593$\pm$0.05&0.148&0.256&0.822$\pm$0.05\\
        \midrule[1pt]
        \multicolumn{4}{l}{\textbf{Epochs}} \\
        \midrule
200 &0.235$\pm$0.02&0.004&0.696&0.861$\pm$0.01\\
300 &0.397$\pm$0.03&0.118&0.960&0.849$\pm$0.04\\
400 &0.508$\pm$0.05&0.114&0.810&0.837$\pm$0.03\\
800 &0.741$\pm$0.04&0.232&0.846&0.860$\pm$0.02\\
1000 &0.775$\pm$0.04&0.216&0.568&0.851$\pm$0.02\\
        \midrule[1pt]
        \multicolumn{4}{l}{\textbf{Weight decay} } \\
        \midrule
        0.0 &0.429$\pm$0.03&0.151&0.300&0.830$\pm$0.03\\
0.0001 &0.563$\pm$0.05&0.134&0.449&0.856$\pm$0.01\\
0.0003 &0.639$\pm$0.05&0.170&0.188&0.841$\pm$0.02\\
0.0005 &0.697$\pm$0.04&0.198&0.124&0.842$\pm$0.01\\
        \midrule[2pt]
        \end{tabular}
}
\label{tab:pws-nasbench101-linear}
\end{table}

\begin{table}[!ht]
% here is the low fidality 
	\caption{\textbf{Results for all low-fidelity factors on the three search spaces.}} 
	\vspace{-0.3cm}
\resizebox{\linewidth}{!}{
	\begin{tabular} { l|cccc}
        \midrule[2pt]
		Factor & \multicolumn{4}{c}{NASBench-101 Chain-like Space} \\
		and & Super-net & \phantom{0} & \phantom{0} & Final \\
		settings & Accuracy & S-KdT & P $>$ R &  Performance \\
        \midrule[1pt]
		\multicolumn{5}{l}{\textbf{Number of layers} (-X indicates the baseline minus X)} \\
		\midrule
Baseline &0.543$\pm$0.05&0.126&0.555&0.863$\pm$0.01\\
-1 &0.734$\pm$0.03&0.184&0.324&0.858$\pm$0.01\\
-2 &0.813$\pm$0.03&0.184&0.270&0.847$\pm$0.02\\
        \midrule[1pt]
		\multicolumn{3}{l}{\textbf{Train portion}} \\
		\midrule
0.25 &0.222$\pm$0.01&0.105&0.542&0.845$\pm$0.02\\
0.5 &0.358$\pm$0.02&0.093&0.696&0.862$\pm$0.01\\
0.75 &0.341$\pm$0.04&0.055&0.308&0.853$\pm$0.01\\
0.9 &0.518$\pm$0.05&0.114&0.136&0.847$\pm$0.01\\        
\midrule[1pt]
		\multicolumn{5}{l}{\textbf{Batch size} (/ X indicates the baseline divided by X)} \\
		\midrule
Baseline &0.566$\pm$0.05&0.158&0.864&0.861$\pm$0.01\\
/2 &0.621$\pm$0.05&0.124&0.920&0.870$\pm$0.01\\
/4 &0.639$\pm$0.06&0.183&0.494&0.848$\pm$0.01\\
        \midrule[1pt]
		\multicolumn{5}{l}{\textbf{\# channels} (/ X indicates the baseline divided by X)} \\
		\midrule
Baseline &0.561$\pm$0.05&0.146&0.864&0.866$\pm$0.01\\
/2 &0.554$\pm$0.05&0.158&0.407&0.843$\pm$0.02\\
/4 &0.435$\pm$0.03&0.153&0.102&0.826$\pm$0.04\\
        \midrule[2pt]
	\end{tabular}
}
\label{tab:supp-lowfd-nb101-linear}
\end{table}

% Below, we provide additional details about our implementations and settings. 

% % \subsection{Cost of Computing the Stand-alone Accuracy}
% % \label{apdx:costSAA}
% % Computing the final accuracy is more expensive than training the super-net. Despite the low-fidelity heuristics reducing the weight-sharing costs, training a stand-alone network to convergence has higher cost, e.g., DARTS searches for 50 epochs but trains from scratch for 600 epochs~\cite{Liu2018darts}. Furthermore, debugging and hyper-parameter tuning typically require training thousands of stand-alone models. Note that, as one typically evaluates a random subset of architectures to understand the design space~\cite{radosavovic_network_2019}, \skdt{} can be computed without additional costs. In any event, the budget for \skdt{} is bounded with $n$.
